# Supplementary material for: Calibrating Predictions to Decisions: A Novel Approach to Multi-Class Calibration
Source: arXiv:2107.05719 source file (2021-07-12)
Supplement: Supplementary file 1 [file appendix.tex]

\section{Additional Results}

\paragraph{Counter Examples} For classwise calibration, construct a very simple example where a prediction function is classwise calibrated but not decision calibrated. In particular, consider $\Yc = \lbrace 0, 1, 2 \rbrace$ and $\Ac = \lbrace 0, 1, 2 \rbrace$. The loss matrix is given by 
\begin{align*}
    \ell(y, a) = \left( \begin{array}{ccc} 0 & -1000 & -1 \\ -1 & 0 & -1000 \\ -1000 & -1 & 0 \end{array} \right) 
\end{align*}
In words, there is a big loss if (y, a) = (0,1), (1, 2) or (2,0) and only a small loss for other types of errors. Consider the prediction function with calibration diagram in Figure~\ref{fig:classwise_example}. Both scenarios are classwise calibrated, but the corresponding (true) decision loss can be drastically different. 

\begin{figure}
    \centering
    \includegraphics[width=0.7\linewidth]{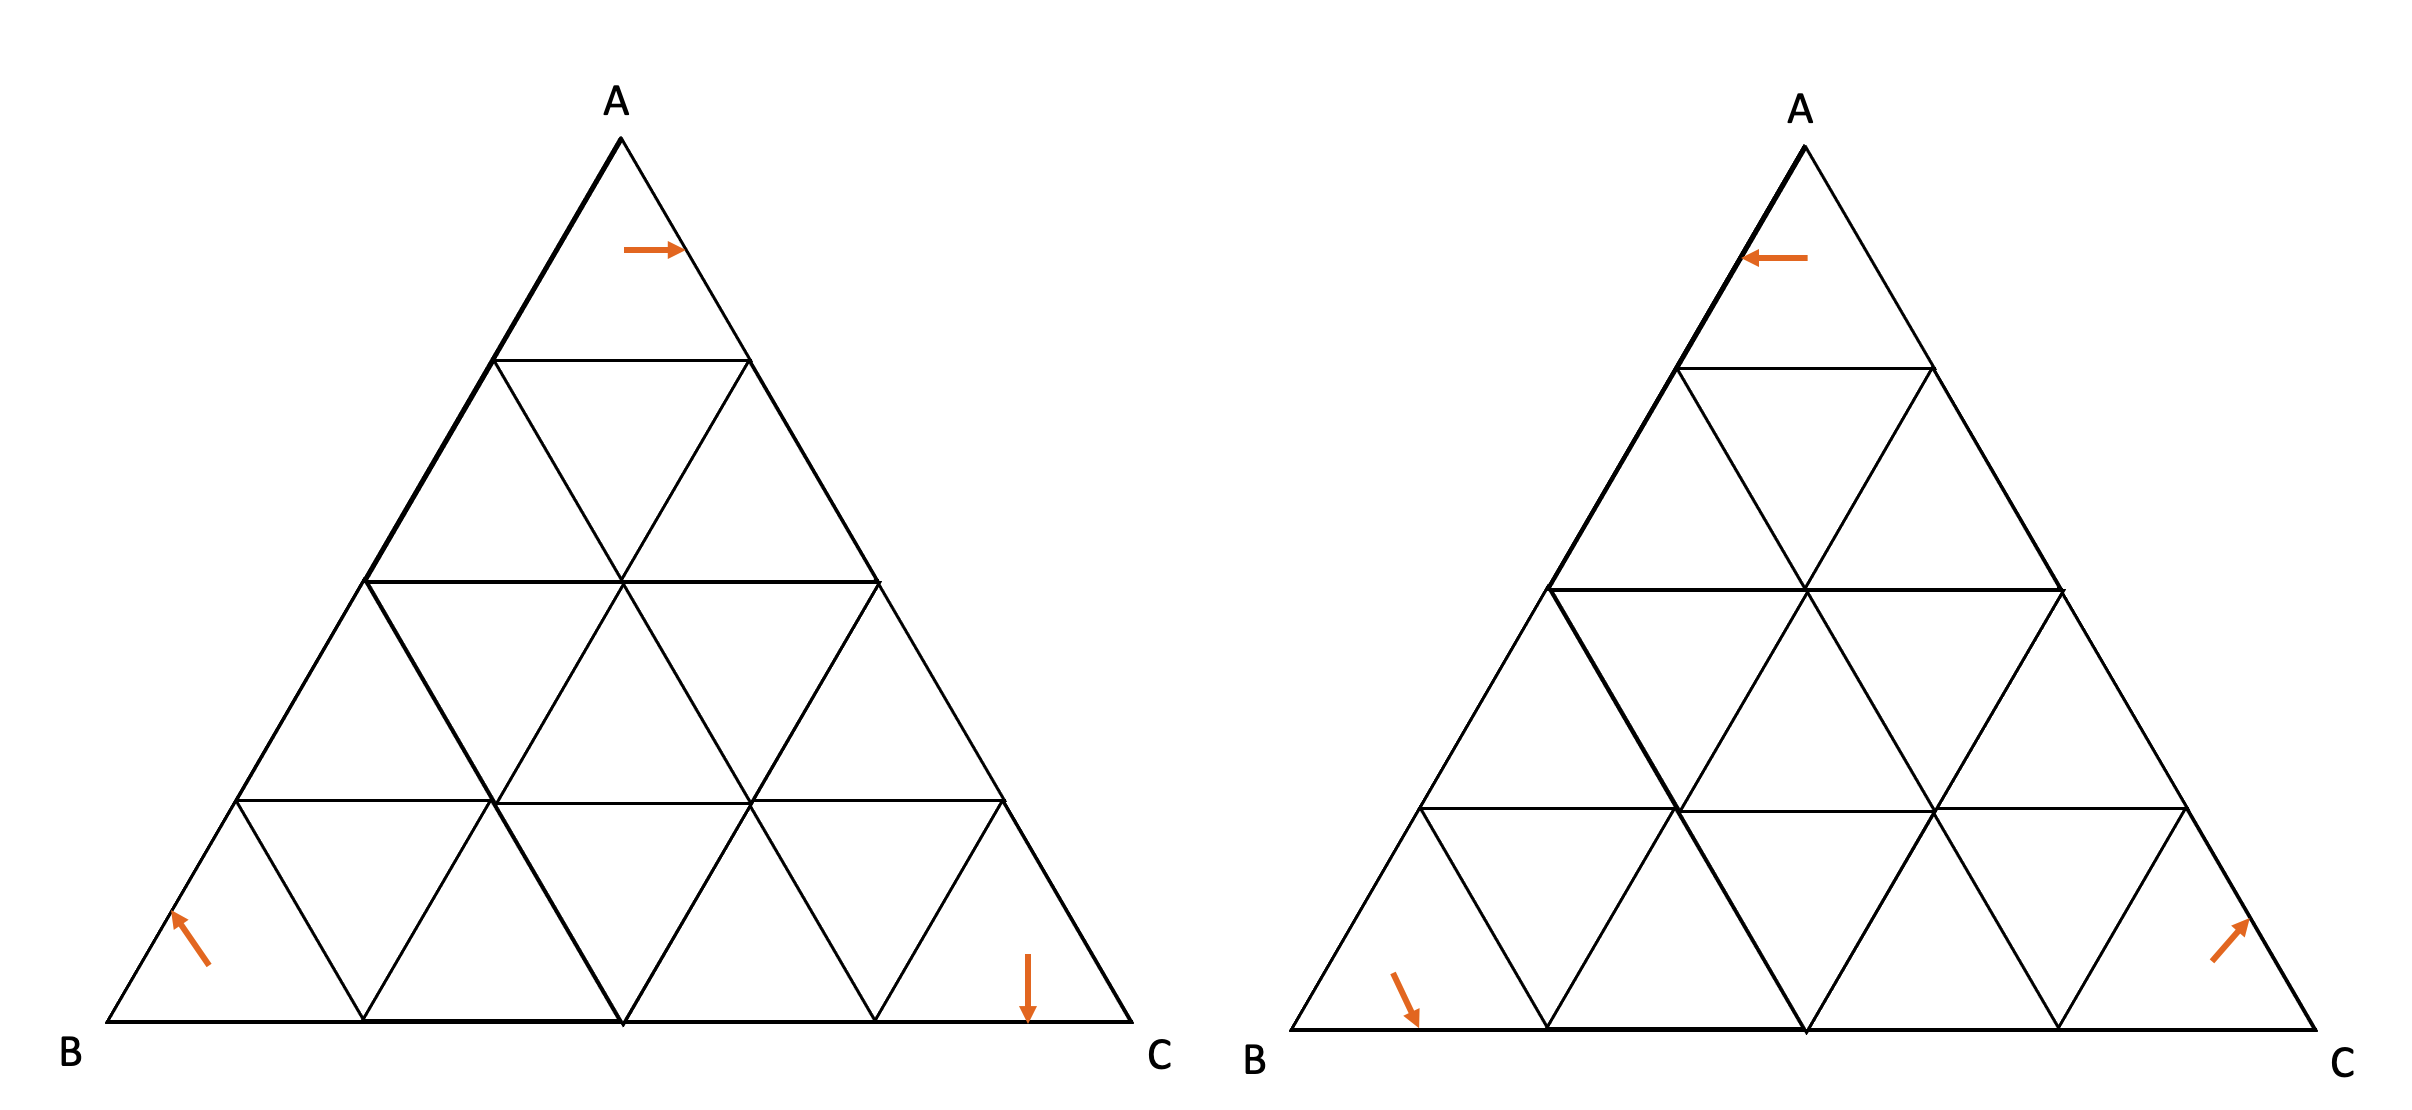}
    \caption{Classwise Calibration counter example}
    \label{fig:classwise_example}
\end{figure}

A forecaster that is classwise calibrated might not be calibrated for a coarsened class (e.g. construct a new classifier where the class poodle and retriever are merged into the same class dog). In the probability simplex this corresponds to orthogonal projection. For example, suppose there are four classes A,B,C,D. when $p(A \mid X) = 0.1$ we always have under $\hp$ $A=0.1,B=0.0$ and when $\hp(A \mid X) = 0.1$ we always have under $\hp$ $A=0.0, B=0.1$, but under $p^*$ $A=0.1, B=0.1$. It is possible to construct such a prediction function that satisfies classwise calibration if there are at least four classes. However if we merge $A,B$ then $\hp(\lbrace A, B \rbrace \mid X) = 0.1$ we have $p^*(\lbrace A, B \rbrace \mid X) = 0.2$. This is no longer classwise calibrated. 

A forecaster that is confidence calibrated might not be calibrated for a coarsened class.

\subsection{Ideas}

In a cancer risk prediction, a image could be classified by different risk groups. There is a provider that offers the prediction function. The loss function depends on the treatment/diagnosis options available at a location or time period. For example, maybe the introduction of a new imaging device could reduce the cost of a false positive: what previous requires an invasive procedure now only requires a easier test. The prediction function does not have to be adjusted depending on the loss function. Instead all the hospitals that use the prediction can know that the computed decision loss equals the true decision loss. 

The loss could depend on some additional variable $U$ but the requirement is that $U$ should be independent of $X$. Often this requires a leap of faith and the assumptions are only approximately true. For example, the prediction of medical images should be independent of the socio-economic status of a person; the prediction of traffic sign in autonomous driving should be independent of the

Suppose there is some "safe" action $a_0$ (such as a conservative treatment, or querying a human) such that $\forall y \in \Yc$ we have $\ell(y, a_0) \geq c$. Then we know that if the prediction function is calibrated, then 
\begin{align*}
    \Eb[\ell(Y, \delta_*(X))] =  \Eb[\ell(\aY, \delta_*(X))]  \geq \inf_y \ell(y, a_0)  \geq c
\end{align*}
